# Supplementary material for: An efficient forgetting-aware fine-tuning framework for pretrained universal machine-learning interatomic potentials
Source: arXiv:2506.15223 ancillary file (2025-06-18)
Supplement: Supplementary file 1 [file FT-supplementary.pdf]

# Supplementary Information

# An efficient forgetting-aware fine-tuning framework for pretrained universal machine-learning interatomic potentials

Jisu Kim[1†], Jiho Lee[1†], Sangmin Oh[1], Yutack Park[1], Seungwoo Hwang[1], Seungwu Han[1,2], Sungwoo Kang[3,4*], Youngho Kang[5*]

*[1]Department of Materials Science and Engineering, Seoul National University, Seoul, 08826, Republic of Korea*
*[2]AI center, Korea Institute of Advanced Study, Seoul, 02455, Republic of Korea*
*[3]Computational Science Research Center, Korea Institute of Science and Technology (KIST), Seoul, 02792, Republic of Korea*
*[4]Division of Nanoscience and Technology, KIST School, University of Science and Technology (UST), Seoul, 02792, Republic of Korea*
*[5]Department of Materials Science and Engineering, Incheon National University, Incheon, 22012, Republic of Korea*

[†] These authors contributed equally to this work
[*] Corresponding authors: sun.w.kang@kist.re.kr and youngho84@inu.ac.kr

## Supplementary Note 1.

**Construction of a Li-Focused Replay set.** To further assess the effect of Replay set on continual learning performance, we construct an additional Li-focused Replay set that covers a narrower chemical space compared to sMPtrj dataset, targeting only Li-containing compounds. To build this Li-focused Replay set for training, we followed the filtering methodology proposed in Ref [1]. Specifically, we first filter Li-containing compounds from the MPtrj training set based on their computed properties and chemical composition. Compounds with a computed bandgap below 2 eV or those containing elements unsuitable for SSEs, such as hydrogen and redox-active elements (V, Cr, Mn, Fe, Co, Ni, and Cu), are removed. These elements are excluded to ensure chemical stability and to avoid undesired effects such as protonic conduction (from hydrogen) or redox reactions (from transition metals).

## Supplementary Figures.

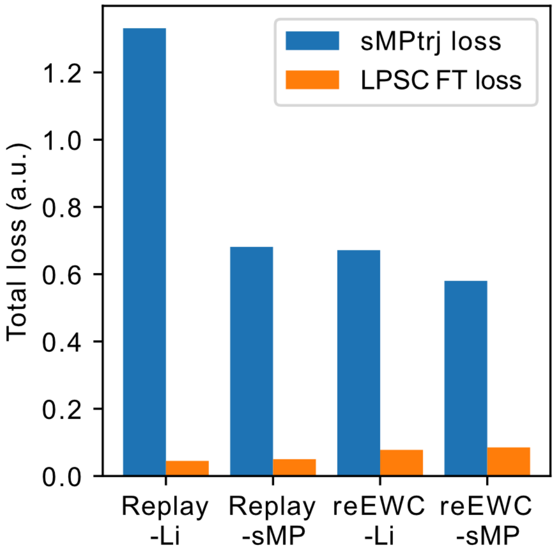


**Supplementary Fig. 1 | Sensitivity of replay set.** The -Li label denotes the Replay set derived from a Li-focused dataset, while -sMP corresponds to a Replay set sampled from the MPtrj dataset. Models fine-tuned with the -Li Replay set show a marked increase in forgetting, likely due to the limited diversity of the Replay data. This highlights the high sensitivity of the standard Replay approach to the choice of Replay set. In contrast, the reEWC method achieves similar loss with both -Li and -sMP Replay sets, indicating its robustness to Replay data set and its effectiveness in mitigating forgetting.

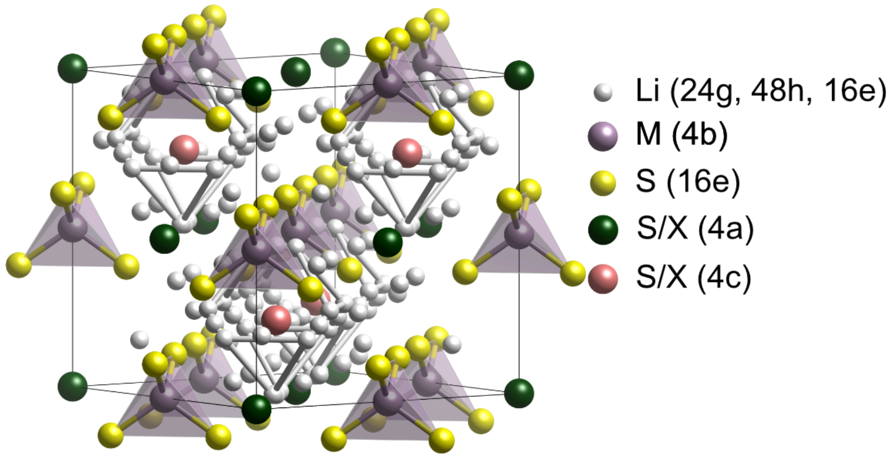


**Supplementary Fig. 2 | Structure of the argyrodite ($Li_{24+x}M_4S_{20}X_4$) unit cell.** Lithium atoms occupy the 24g, 48h and 16e sites, while metal cations (*M*=P, As, Sb, Si, Ge, and Si) are located at 4b sites, forming $MS_4$ tetrahedra with sulfur at the 16e positions. The 4a and 4c sites are shared by sulfur ($S^-$) and halide ($X^-$=$Cl^-$, $Br^-$, and $I^-$) anions, resulting in anion-site disorder (S/*X* disorder). In the argyrodite-type test set, various levels of S/*X* disorder (0%, 25%, 50%, 75%, and 100% *X*@4c) are considered. For the fine-tuning set based on $Li_{24}P_4S_{20}Cl_4$, a configuration with 50% Cl@4c is used, where two Cl atoms occupy the 4a and 4c sites, and the remaining positions are filled by S atoms.

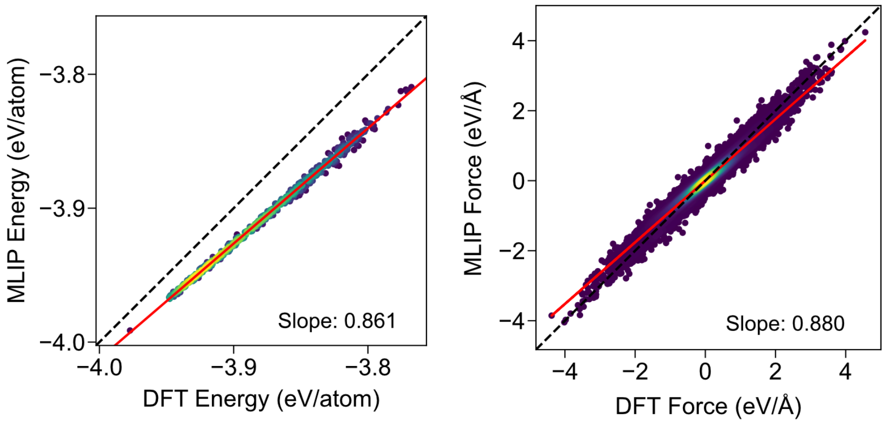


**Supplementary Fig. 3 | Definition of softening scale based on energy and force parity plots for $Li_{6.25}As_{0.25}Ge_{0.25}P_{0.25}Sb_{0.25}Cl_{0.25}I_{0.75}$, comparing DFT and SevenNet-0 results.** The slope (red line), representing the softening scale, is obtained via linear fitting of the data points and is shown in the lower-right corner. A slope value less than 1 indicates softening, while a value greater than 1 indicates stiffening.

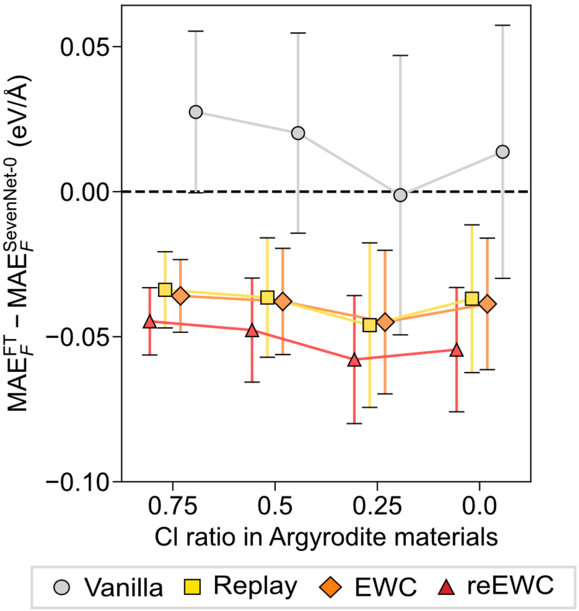


**Supplementary Fig. 4 | Assessment of knowledge transfer with respect to the Cl ratio in argyrodite materials.** Changes in force mean absolute error (MAE) relative to SevenNet-0 across argyrodite-type test materials, grouped by the ratio of chlorine (Cl). Each data point represents the average force MAE change for materials at a given Cl ratio, with error bars indicating the standard deviation. A Cl ratio of 1 corresponds to $Li_6PS_5Cl$ (LPSC), included in the fine-tuning set. Decreasing Cl ratios indicate non-Cl argyrodite structures, representing compositions increasingly distant from the LPSC fine-tuning set. Gray circle, yellow square, orange diamond, and red triangle markers correspond to vanilla, replay, EWC, and reEWC MLIPs, respectively.

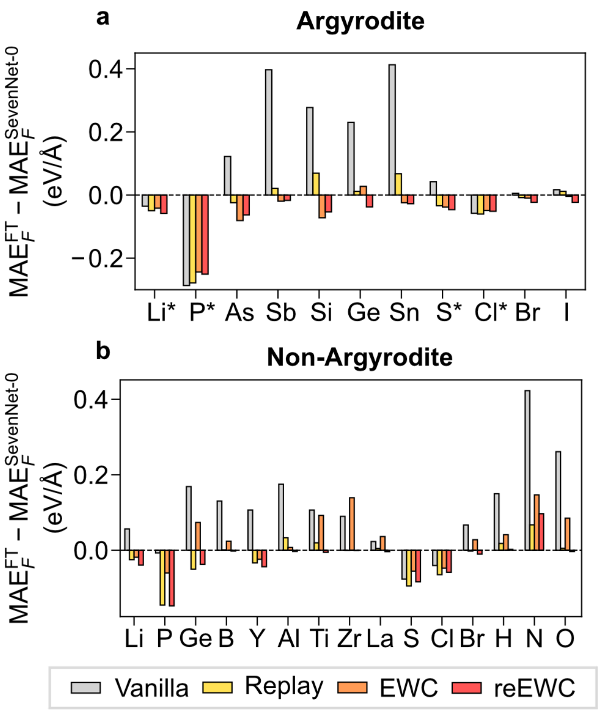


**Supplementary Fig. 5 | Quantification of MLIP forgetting through force accuracy across element types.** Element-wise averaged force MAE relative to SevenNet-0 for **a** 126 argyrodite-type materials and **b** 9 non-argyrodite-type materials. Histograms show the average force MAE change for each element, calculated as the difference between the force MAE of each MLIP and SevenNet-0. Positive values indicate forgetting, while negative values reflect effective forgetting prevention and knowledge transfer. Asterisks indicate elements (Li, P, S, Cl) included in the LPSC fine-tuning set. Gray, yellow, orange, and red bars represent Vanilla, Replay, EWC, and reEWC MLIPs, respectively.

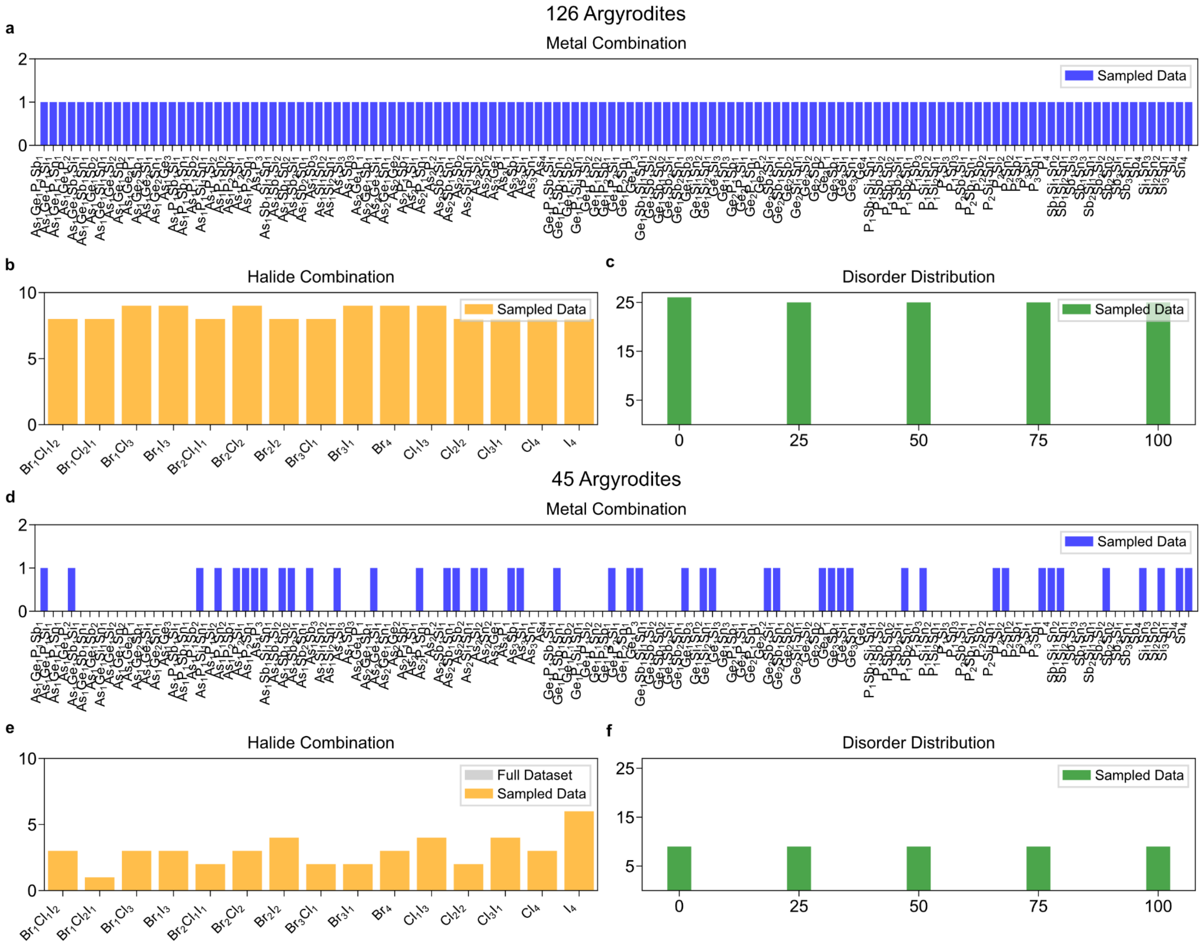


**Supplementary Fig. 6 | Distribution of metal, halide and disorder in argyrodite structures for potential validation and diffusivity calculation. a–c** Distribution of 126 representative argyrodite structures used for potential energy surface evaluation, categorized by metal combinations, halide combinations, and disorder, respectively. **d–f** Distribution of 45 representative argyrodite structures used for diffusivity calculations, categorized by metal combinations, halide combinations, and disorder, respectively.

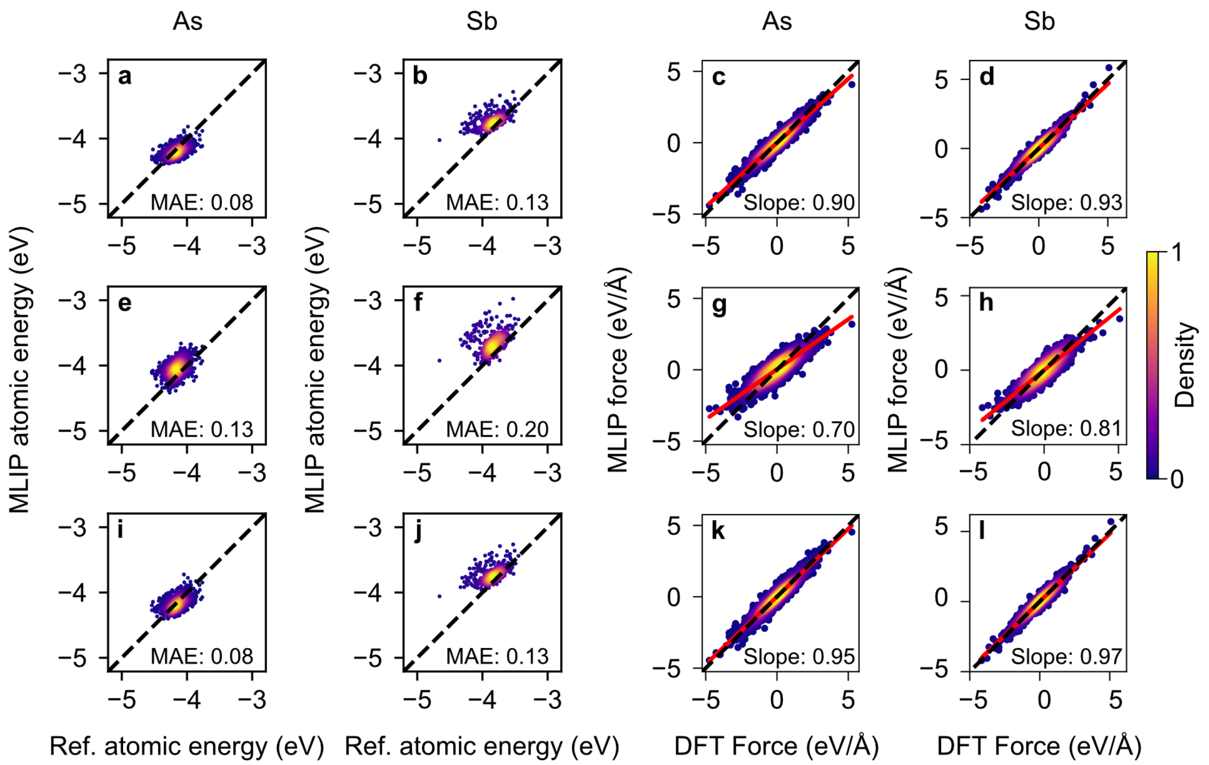


**Supplementary Fig. 7 | Dynamical behavior of $Li_6As_{0.75}Sb_{0.25}S_5Br_{0.5}I_{0.5}$ for As and Sb atoms. a-l** Parity plots comparing predicted and reference values for As and Sb atoms: **a-d** SevenNet-0, **e-h** Vanilla MLIP, and **i-l** reEWC MLIP. Atomic energy predictions are shown in **a,e,i** (As) and **b,f,j** (Sb), with mean absolute error (MAE) values in eV displayed in each plot. Atomic force predictions are shown in **c,g,k** (As) and **d,h,l** (Sb), with red lines indicating the slope (values in lower-right corner). Vanilla MLIP exhibits significant performance degradation in both atomic energies and forces, with notable force softening indicating catastrophic forgetting. In contrast, reEWC MLIP maintains atomic energy accuracy comparable to SevenNet-0 while showing improved atomic force predictions for both As and Sb atoms.

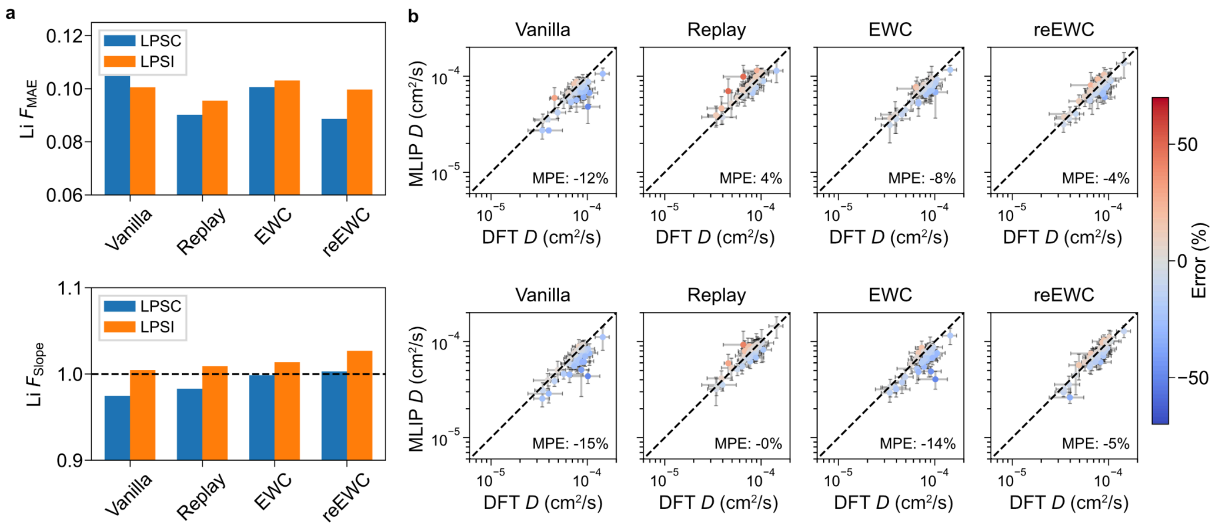


**Supplementary Fig. 8 | Impact of fine-tuning set selection on force accuracy and Li diffusivity predictions.** **a** Comparison of fine-tuned MLIPs using two different fine-tuning sets—LPSC (600, 1000 K AIMD of $Li_6PS_5Cl$) and LPSI (600 K AIMD of $Li_6PS_5I$)—evaluated on 45 argyrodite materials at 1200 K. Top: Mean absolute error (MAE) in Li forces with respect to DFT. LPSI fine-tuned MLIPs generally show increased force MAEs, indicating degraded transferability. Bottom: Force parity slopes, where systematically higher slopes for LPSI fine-tuned MLIPs suggest PES stiffening due to overfitting to low-diffusivity LPSI configurations. **b**, Scatter plots of Li diffusivity at 1200 K predicted by the same fine-tuned MLIPs. Top: Results from LPSC fine-tuning set. Bottom: Results from LPSI fine-tuning set. Fine-tuning with the LPSI set results in consistently underestimated diffusivities, with reduced mean percentage error (MPE) indicating suppression of inter-cage hopping events. These trends highlight the importance of selecting diverse, high-diffusivity configurations to avoid PES over-constraining and ensure accurate transport predictions.

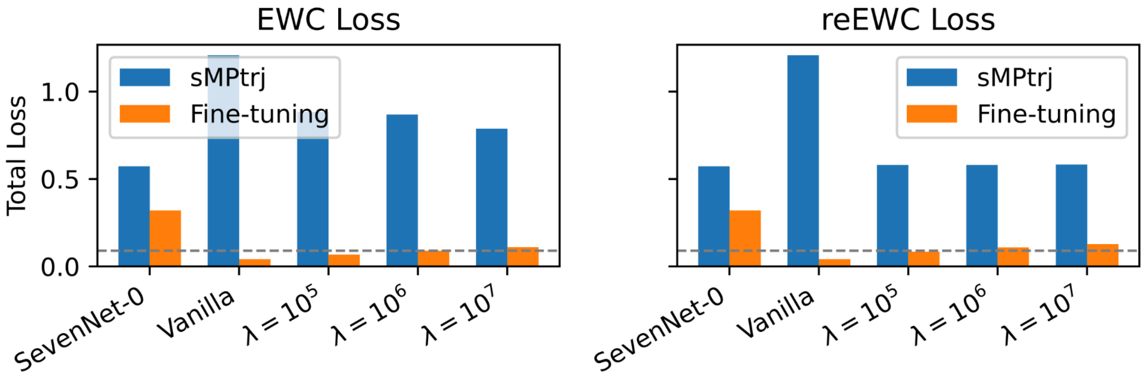


**Supplementary Fig. 9 | Total loss on the fine-tuning set and sMPtrj as a function of the regularization strength ($\lambda$) for EWC and reEWC models.** The fine-tuning set loss indicates how well each model adapts to the target system ($Li_6PS_5Cl$), while the sMPtrj loss measures the degree of forgetting on the pretrained dataset. The Vanilla MLIP achieves low fine-tuning loss but suffers substantial forgetting. In contrast, both EWC and reEWC models achieve competitive target accuracy while significantly mitigating forgetting. For the EWC MLIP, ($\lambda = 10^6$) is selected as the optimal value, balancing a fine-tuning loss with a reduced sMPtrj loss. For reEWC, ($\lambda = 10^5$) is found to be sufficient, achieving low loss both on the fine-tuning set and sMPtrj. The horizontal dashed line denotes the target loss threshold (0.09) used to guide ($\lambda$) selection.

**Supplementary Table. 1 | Detailed information for 126 argyrodite-type test structures**

| Composition | Metal | Halide | Disorder (%) | Diffusivity Calculation |
|---|---|---|---|---|
| Li6.25As0.25Ge0.25P0.25Sb0.25S5.00Cl0.25I0.75 | As1Ge1P1Sb1 | Cl1I3 | 25 | O |
| Li6.50As0.25Ge0.25P0.25Si0.25S5.00Br0.75I0.25 | As1Ge1P1Si1 | Br3I1 | 75 | X |
| Li6.50As0.25Ge0.25P0.25Sn0.25S5.00Cl0.50I0.50 | As1Ge1P1Sn1 | Cl2I2 | 25 | X |
| Li6.25As0.25Ge0.25P0.50S5.00Cl0.25I0.75 | As1Ge1P2 | Cl1I3 | 75 | O |
| Li6.50As0.25Ge0.25Sb0.25Si0.25S5.00Cl0.50I0.50 | As1Ge1Sb1Si1 | Cl2I2 | 75 | X |
| Li6.50As0.25Ge0.25Sb0.25Sn0.25S5.00Br0.50Cl0.25I0.25 | As1Ge1Sb1Sn1 | Br2Cl1I1 | 0 | X |
| Li6.25As0.25Ge0.25Sb0.50S5.00Br0.75Cl0.25 | As1Ge1Sb2 | Br3Cl1 | 50 | X |
| Li6.75As0.25Ge0.25Si0.25Sn0.25S5.00Cl1.00 | As1Ge1Si1Sn1 | Cl4 | 100 | X |
| Li6.75As0.25Ge0.25Si0.50S5.00Br0.50Cl0.25I0.25 | As1Ge1Si2 | Br2Cl1I1 | 50 | X |
| Li6.75As0.25Ge0.25Sn0.50S5.00Cl0.75I0.25 | As1Ge1Sn2 | Cl3I1 | 50 | X |
| Li6.50As0.25Ge0.50P0.25S5.00Cl0.75I0.25 | As1Ge2P1 | Cl3I1 | 75 | X |
| Li6.50As0.25Ge0.50Sb0.25S5.00Cl1.00 | As1Ge2Sb1 | Cl4 | 50 | X |
| Li6.75As0.25Ge0.50Si0.25S5.00Br1.00 | As1Ge2Si1 | Br4 | 0 | X |
| Li6.75As0.25Ge0.50Sn0.25S5.00Br0.25Cl0.50I0.25 | As1Ge2Sn1 | Br1Cl2I1 | 75 | X |
| Li6.75As0.25Ge0.75S5.00Cl0.25I0.75 | As1Ge3 | Cl1I3 | 50 | X |
| Li6.25As0.25P0.25Sb0.25Si0.25S5.00Cl1.00 | As1P1Sb1Si1 | Cl4 | 0 | X |
| Li6.25As0.25P0.25Sb0.25Sn0.25S5.00Br0.25Cl0.50I0.25 | As1P1Sb1Sn1 | Br1Cl2I1 | 50 | X |
| Li6.00As0.25P0.25Sb0.50S5.00Br0.25Cl0.25I0.50 | As1P1Sb2 | Br1Cl1I2 | 75 | O |
| Li6.50As0.25P0.25Si0.25Sn0.25S5.00Br0.25Cl0.75 | As1P1Si1Sn1 | Br1Cl3 | 25 | X |
| Li6.50As0.25P0.25Si0.50S5.00Cl0.75I0.25 | As1P1Si2 | Cl3I1 | 25 | O |
| Li6.50As0.25P0.25Sn0.50S5.00Br0.25Cl0.25I0.50 | As1P1Sn2 | Br1Cl1I2 | 25 | X |
| Li6.00As0.25P0.50Sb0.25S5.00I1.00 | As1P2Sb1 | I4 | 75 | O |
| Li6.25As0.25P0.50Si0.25S5.00Cl0.25I0.75 | As1P2Si1 | Cl1I3 | 0 | O |
| Li6.25As0.25P0.50Sn0.25S5.00Br1.00 | As1P2Sn1 | Br4 | 0 | O |
| Li6.00As0.25P0.75S5.00Cl1.00 | As1P3 | Cl4 | 100 | O |
| Li6.50As0.25Sb0.25Si0.25Sn0.25S5.00Br0.50Cl0.50 | As1Sb1Si1Sn1 | Br2Cl2 | 50 | X |

| | | | | |
|---|---|---|---|---|
| Li6.50As0.25Sb0.25Si0.50S5.00Br1.00 | As1Sb1Si2 | Br4 | 75 | O |
| Li6.50As0.25Sb0.25Sn0.50S5.00Br0.50Cl0.50 | As1Sb1Sn2 | Br2Cl2 | 50 | O |
| Li6.25As0.25Sb0.50Si0.25S5.00Br0.25Cl0.75 | As1Sb2Si1 | Br1Cl3 | 50 | X |
| Li6.25As0.25Sb0.50Sn0.25S5.00Br0.25I0.75 | As1Sb2Sn1 | Br1I3 | 100 | O |
| Li6.00As0.25Sb0.75S5.00Cl0.50I0.50 | As1Sb3 | Cl2I2 | 0 | X |
| Li6.75As0.25Si0.25Sn0.50S5.00Cl0.50I0.50 | As1Si1Sn2 | Cl2I2 | 75 | X |
| Li6.75As0.25Si0.50Sn0.25S5.00Cl0.75I0.25 | As1Si2Sn1 | Cl3I1 | 0 | O |
| Li6.75As0.25Si0.75S5.00Br1.00 | As1Si3 | Br4 | 50 | X |
| Li6.75As0.25Sn0.75S5.00Br0.75Cl0.25 | As1Sn3 | Br3Cl1 | 100 | X |
| Li6.25As0.50Ge0.25P0.25S5.00Br0.50Cl0.25I0.25 | As2Ge1P1 | Br2Cl1I1 | 25 | X |
| Li6.25As0.50Ge0.25Sb0.25S5.00Br0.50Cl0.50 | As2Ge1Sb1 | Br2Cl2 | 75 | O |
| Li6.50As0.50Ge0.25Si0.25S5.00Br0.50Cl0.50 | As2Ge1Si1 | Br2Cl2 | 25 | X |
| Li6.50As0.50Ge0.25Sn0.25S5.00Br0.25I0.75 | As2Ge1Sn1 | Br1I3 | 0 | X |
| Li6.50As0.50Ge0.50S5.00Br0.50I0.50 | As2Ge2 | Br2I2 | 75 | X |
| Li6.00As0.50P0.25Sb0.25S5.00Br0.25Cl0.25I0.50 | As2P1Sb1 | Br1Cl1I2 | 50 | X |
| Li6.25As0.50P0.25Si0.25S5.00Cl0.50I0.50 | As2P1Si1 | Cl2I2 | 50 | O |
| Li6.25As0.50P0.25Sn0.25S5.00Br0.25Cl0.75 | As2P1Sn1 | Br1Cl3 | 75 | X |
| Li6.00As0.50P0.50S5.00Br0.75Cl0.25 | As2P2 | Br3Cl1 | 100 | X |
| Li6.25As0.50Sb0.25Si0.25S5.00Br0.50I0.50 | As2Sb1Si1 | Br2I2 | 100 | O |
| Li6.25As0.50Sb0.25Sn0.25S5.00I1.00 | As2Sb1Sn1 | I4 | 25 | O |
| Li6.00As0.50Sb0.50S5.00Br0.25Cl0.50I0.25 | As2Sb2 | Br1Cl2I1 | 75 | X |
| Li6.50As0.50Si0.25Sn0.25S5.00Cl0.75I0.25 | As2Si1Sn1 | Cl3I1 | 0 | O |
| Li6.50As0.50Si0.50S5.00Cl0.50I0.50 | As2Si2 | Cl2I2 | 75 | O |
| Li6.50As0.50Sn0.50S5.00Br0.25I0.75 | As2Sn2 | Br1I3 | 0 | X |
| Li6.25As0.75Ge0.25S5.00Br0.50Cl0.25I0.25 | As3Ge1 | Br2Cl1I1 | 75 | X |
| Li6.00As0.75P0.25S5.00Br0.25I0.75 | As3P1 | Br1I3 | 25 | O |
| Li6.00As0.75Sb0.25S5.00Br0.50I0.50 | As3Sb1 | Br2I2 | 100 | O |
| Li6.25As0.75Si0.25S5.00I1.00 | As3Si1 | I4 | 50 | X |
| Li6.25As0.75Sn0.25S5.00Br0.25Cl0.75 | As3Sn1 | Br1Cl3 | 75 | X |

| | | | | |
|---|---|---|---|---|
| Li6.00As1.00S5.00Br0.25Cl0.25I0.50 | As4 | Br1Cl1I2 | 25 | X |
| Li6.50Ge0.25P0.25Sb0.25Si0.25S5.00I1.00 | Ge1P1Sb1Si1 | I4 | 0 | O |
| Li6.50Ge0.25P0.25Sb0.25Sn0.25S5.00Br0.50Cl0.25I0.25 | Ge1P1Sb1Sn1 | Br2Cl1I1 | 100 | X |
| Li6.25Ge0.25P0.25Sb0.50S5.00Br0.75I0.25 | Ge1P1Sb2 | Br3I1 | 25 | X |
| Li6.75Ge0.25P0.25Si0.25Sn0.25S5.00I1.00 | Ge1P1Si1Sn1 | I4 | 25 | X |
| Li6.75Ge0.25P0.25Si0.50S5.00Br0.75I0.25 | Ge1P1Si2 | Br3I1 | 100 | X |
| Li6.75Ge0.25P0.25Sn0.50S5.00Br0.25Cl0.25I0.50 | Ge1P1Sn2 | Br1Cl1I2 | 75 | X |
| Li6.25Ge0.25P0.50Sb0.25S5.00Br0.25I0.75 | Ge1P2Sb1 | Br1I3 | 0 | O |
| Li6.50Ge0.25P0.50Si0.25S5.00Br0.75Cl0.25 | Ge1P2Si1 | Br3Cl1 | 0 | X |
| Li6.50Ge0.25P0.50Sn0.25S5.00Br0.50Cl0.50 | Ge1P2Sn1 | Br2Cl2 | 100 | O |
| Li6.25Ge0.25P0.75S5.00Br0.25Cl0.25I0.50 | Ge1P3 | Br1Cl1I2 | 50 | O |
| Li6.75Ge0.25Sb0.25Si0.25Sn0.25S5.00Br0.25I0.75 | Ge1Sb1Si1Sn1 | Br1I3 | 100 | X |
| Li6.75Ge0.25Sb0.25Si0.50S5.00Cl1.00 | Ge1Sb1Si2 | Cl4 | 100 | X |
| Li6.75Ge0.25Sb0.25Sn0.50S5.00Br0.50I0.50 | Ge1Sb1Sn2 | Br2I2 | 0 | X |
| Li6.50Ge0.25Sb0.50Si0.25S5.00Br0.50I0.50 | Ge1Sb2Si1 | Br2I2 | 100 | X |
| Li6.50Ge0.25Sb0.50Sn0.25S5.00Br0.50I0.50 | Ge1Sb2Sn1 | Br2I2 | 25 | O |
| Li6.25Ge0.25Sb0.75S5.00Br0.50Cl0.50 | Ge1Sb3 | Br2Cl2 | 75 | X |
| Li7.00Ge0.25Si0.25Sn0.50S5.00Br0.25Cl0.75 | Ge1Si1Sn2 | Br1Cl3 | 75 | O |
| Li7.00Ge0.25Si0.50Sn0.25S5.00Br0.75Cl0.25 | Ge1Si2Sn1 | Br3Cl1 | 100 | O |
| Li7.00Ge0.25Si0.75S5.00Br0.50I0.50 | Ge1Si3 | Br2I2 | 100 | X |
| Li7.00Ge0.25Sn0.75S5.00I1.00 | Ge1Sn3 | I4 | 50 | X |
| Li6.50Ge0.50P0.25Sb0.25S5.00Br0.75I0.25 | Ge2P1Sb1 | Br3I1 | 100 | X |
| Li6.75Ge0.50P0.25Si0.25S5.00Cl1.00 | Ge2P1Si1 | Cl4 | 25 | X |
| Li6.75Ge0.50P0.25Sn0.25S5.00Cl0.25I0.75 | Ge2P1Sn1 | Cl1I3 | 0 | X |
| Li6.50Ge0.50P0.50S5.00I1.00 | Ge2P2 | I4 | 0 | O |
| Li6.75Ge0.50Sb0.25Si0.25S5.00Cl1.00 | Ge2Sb1Si1 | Cl4 | 100 | O |
| Li6.75Ge0.50Sb0.25Sn0.25S5.00Cl0.25I0.75 | Ge2Sb1Sn1 | Cl1I3 | 25 | X |
| Li6.50Ge0.50Sb0.50S5.00Cl1.00 | Ge2Sb2 | Cl4 | 75 | X |
| Li7.00Ge0.50Si0.25Sn0.25S5.00Br0.75Cl0.25 | Ge2Si1Sn1 | Br3Cl1 | 0 | X |

| | | | | |
|---|---|---|---|---|
| Li7.00Ge0.50Si0.50S5.00Br0.25I0.75 | Ge2Si2 | Br1I3 | 25 | X |
| Li7.00Ge0.50Sn0.50S5.00Br0.50I0.50 | Ge2Sn2 | Br2I2 | 75 | O |
| Li6.75Ge0.75P0.25S5.00Br0.75Cl0.25 | Ge3P1 | Br3Cl1 | 25 | O |
| Li6.75Ge0.75Sb0.25S5.00Br0.25Cl0.75 | Ge3Sb1 | Br1Cl3 | 75 | O |
| Li7.00Ge0.75Si0.25S5.00Br0.25Cl0.50I0.25 | Ge3Si1 | Br1Cl2I1 | 0 | O |
| Li7.00Ge0.75Sn0.25S5.00Br0.25Cl0.50I0.25 | Ge3Sn1 | Br1Cl2I1 | 75 | X |
| Li7.00Ge1.00S5.00Br1.00 | Ge4 | Br4 | 100 | X |
| Li6.50P0.25Sb0.25Si0.25Sn0.25S5.00Br0.50I0.50 | P1Sb1Si1Sn1 | Br2I2 | 0 | X |
| Li6.50P0.25Sb0.25Si0.50S5.00Br0.25I0.75 | P1Sb1Si2 | Br1I3 | 100 | X |
| Li6.50P0.25Sb0.25Sn0.50S5.00Cl0.75I0.25 | P1Sb1Sn2 | Cl3I1 | 0 | X |
| Li6.25P0.25Sb0.50Si0.25S5.00Br0.25Cl0.75 | P1Sb2Si1 | Br1Cl3 | 50 | O |
| Li6.25P0.25Sb0.50Sn0.25S5.00Br0.50Cl0.50 | P1Sb2Sn1 | Br2Cl2 | 75 | X |
| Li6.00P0.25Sb0.75S5.00Br0.25Cl0.25I0.50 | P1Sb3 | Br1Cl1I2 | 100 | O |
| Li6.75P0.25Si0.25Sn0.50S5.00Br1.00 | P1Si1Sn2 | Br4 | 0 | X |
| Li6.75P0.25Si0.50Sn0.25S5.00Cl0.75I0.25 | P1Si2Sn1 | Cl3I1 | 50 | X |
| Li6.75P0.25Si0.75S5.00Cl0.50I0.50 | P1Si3 | Cl2I2 | 0 | X |
| Li6.75P0.25Sn0.75S5.00Cl0.50I0.50 | P1Sn3 | Cl2I2 | 50 | X |
| Li6.25P0.50Sb0.25Si0.25S5.00Br0.25Cl0.50I0.25 | P2Sb1Si1 | Br1Cl2I1 | 25 | X |
| Li6.25P0.50Sb0.25Sn0.25S5.00Br0.50Cl0.25I0.25 | P2Sb1Sn1 | Br2Cl1I1 | 100 | X |
| Li6.00P0.50Sb0.50S5.00Br0.50Cl0.50 | P2Sb2 | Br2Cl2 | 75 | X |
| Li6.50P0.50Si0.25Sn0.25S5.00Br0.50Cl0.25I0.25 | P2Si1Sn1 | Br2Cl1I1 | 100 | O |
| Li6.50P0.50Si0.50S5.00I1.00 | P2Si2 | I4 | 25 | O |
| Li6.50P0.50Sn0.50S5.00Br1.00 | P2Sn2 | Br4 | 100 | X |
| Li6.00P0.75Sb0.25S5.00Cl0.25I0.75 | P3Sb1 | Cl1I3 | 100 | X |
| Li6.25P0.75Si0.25S5.00Br0.75I0.25 | P3Si1 | Br3I1 | 25 | X |
| Li6.25P0.75Sn0.25S5.00Br1.00 | P3Sn1 | Br4 | 50 | O |
| Li6.00P1.00S5.00Cl1.00 | P4 | Cl4 | 50 | O |
| Li6.75Sb0.25Si0.25Sn0.50S5.00Cl0.25I0.75 | Sb1Si1Sn2 | Cl1I3 | 50 | O |
| Li6.75Sb0.25Si0.50Sn0.25S5.00Br0.25Cl0.50I0.25 | Sb1Si2Sn1 | Br1Cl2I1 | 25 | X |

| | | | | |
|---|---|---|---|---|
| Li6.75Sb0.25Si0.75S5.00Cl0.25I0.75 | Sb1Si3 | Cl1I3 | 100 | X |
| Li6.75Sb0.25Sn0.75S5.00Cl0.75I0.25 | Sb1Sn3 | Cl3I1 | 0 | X |
| Li6.50Sb0.50Si0.25Sn0.25S5.00Br0.25Cl0.50I0.25 | Sb2Si1Sn1 | Br1Cl2I1 | 25 | X |
| Li6.50Sb0.50Si0.50S5.00I1.00 | Sb2Si2 | I4 | 0 | O |
| Li6.50Sb0.50Sn0.50S5.00Br0.75Cl0.25 | Sb2Sn2 | Br3Cl1 | 50 | X |
| Li6.25Sb0.75Si0.25S5.00Br0.25Cl0.75 | Sb3Si1 | Br1Cl3 | 50 | X |
| Li6.25Sb0.75Sn0.25S5.00Br0.25I0.75 | Sb3Sn1 | Br1I3 | 0 | X |
| Li6.00Sb1.00S5.00Cl0.75I0.25 | Sb4 | Cl3I1 | 25 | O |
| Li7.00Si0.25Sn0.75S5.00Br0.25Cl0.25I0.50 | Si1Sn3 | Br1Cl1I2 | 25 | X |
| Li7.00Si0.50Sn0.50S5.00Br0.75I0.25 | Si2Sn2 | Br3I1 | 25 | O |
| Li7.00Si0.75Sn0.25S5.00Br0.75I0.25 | Si3Sn1 | Br3I1 | 0 | X |
| Li7.00Si1.00S5.00Br0.50Cl0.25I0.25 | Si4 | Br2Cl1I1 | 50 | O |
| Li7.00Sn1.00S5.00Br0.75I0.25 | Sn4 | Br3I1 | 50 | O |

# References


1. He, X., Zhu, Y., Epstein, A., Mo, Y.: Statistical variances of diffusional properties from ab initio molecular dynamics simulations. npj Comput. Mater. **4**(1), 18 (2018)
